# Supplementary material for: Multi-Layer Confidence Scoring for Detection of Out-of-Distribution Samples, Adversarial Attacks, and In-Distribution Misclassifications
Source: arXiv:2512.19472 source file (2025-12-22)
Supplement: Supplementary file 1 [file appendix.tex]

\cleardoublepage
\newpage
\appendices

\section{Handling Non-Linear Layers}\label{app: cv computation general}

\subsubsection{Convolutional Layers}\label{subsec: conv layers}

While fully-connected layers can be mapped in $\affineTransform=\left[ \weights | \biases \right]$ form, convolution ones need to be unrolled into an affine format.
To do so, we apply a Toeplitz unrolling of the convolution filters according to \cite{sedghi2018singular,gnacik2022using}.
Consider a convolutional layer $\layer$ with $\convChannelsIn$ input and $\convChannelsOut$ output channels, and a kernel of size $\convKernelHeight\times\convKernelWidth$ for each combination of input and output channels.
Considering $\layer$ to operate on images (or activations) of shape $\convChannelsIn\times\convInputHeight\times\convInputWidth$, yielding to output images of shape $\convChannelsOut\times\convOutputHeight\times\convOutputWidth$\footnote{The output sizes depend on the layer's \codeFont{stride}, \codeFont{padding}, and \codeFont{dilation} parameters.}, the Toeplitz unrolling of the kernels is the matrix $\convToeplitzMatrix\in\realSet^{(\convChannelsOut\times\convOutputHeight\times\convOutputWidth)\times(\convChannelsIn\times\convInputHeight\times\convInputWidth)}$, where each of the $\convChannelsIn\times\convChannelsOut$ blocks corresponds to the Toeplitz unrolling of a single convolution kernel \cite{sedghi2018singular}.

Given a single kernel $\convKernel_{i,j}$ corresponding to the input channel $i\in\{0, \hdots, \convChannelsIn-1\}$ and output channel $j\in\{0, \hdots, \convChannelsOut-1\}$, its Toeplitz unrolling $\convToeplitzMatrix_{i, j}\in\realSet^{(\convOutputHeight\times\convOutputWidth)\times(\convInputHeight\times\convInputWidth)}$ is the double circulant matrix defined by Eq. \eqref{eq: single kernel toeplitz} \cite{sedghi2018singular}, where $\circulant$ is the circulant operator\footnote{On the practical side, the circulant needs to consider the convolution layer's \codeFont{stride}, \codeFont{padding}, and \codeFont{dilation} parameters} and $\convKernel_{i,j}[k,:]$ is the $k-th$ row of $\convKernel_{i,j}$. For readability, we will use the shorthand notation $\convKernel[k]$ to indicate $\circulant(\convKernel_{i,j}[k,:])$ in Eq. \eqref{eq: single kernel toeplitz}.

\begin{multline}\label{eq: single kernel toeplitz}
	\convToeplitzMatrix=\left[
	\begin{array}{cccc}
		\convKernel[0] & \convKernel[1] & \hdots & \convKernel[\convKernelWidth-1] \\
		\convKernel[\convKernelWidth-1] & \convKernel[0] & \hdots & \convKernel[\convKernelWidth-2] \\
		\vdots & \vdots & \ddots & \vdots \\
		\convKernel[1] & \convKernel[2] & \hdots & \convKernel[0] \\
	\end{array}
	\right]
\end{multline}

% \begin{multline}\label{eq: single kernel toeplitz}
	% 	\convToeplitzMatrix_{i, j} = \\
	% 	\left[
	% 	\begin{array}{cccc}
		% 		\circulant(\convKernel_{i,j}[0,:]) & \circulant(\convKernel_{i,j}[1,:]) & \hdots & \circulant(\convKernel_{i,j}[\convKernelWidth-1,:]) \\
		% 		\circulant(\convKernel_{i,j}[\convKernelWidth-1,:]) & \circulant(\convKernel_{i,j}[0,:]) & \hdots & \circulant(\convKernel_{i,j}[\convKernelWidth-2,:]) \\
		% 		\vdots & \vdots & \vdots & \vdots \\
		% 		\circulant(\convKernel_{i,j}[1,:]) & \circulant(\convKernel_{i,j}[2,:]) & \hdots & \circulant(\convKernel_{i,j}[0,:]) \\
		% 	\end{array}
	% 	\right]
	% \end{multline}

With $\convToeplitzMatrix$ in place, the convolution operation performed by $\layer$ can be written as $\flatten(\actOut) = \flatten(\layer(\actIn)) = \convToeplitzMatrix\flatten(\actIn)$, where the $\flatten$ operator transforms input and output activations, $\actIn$ and $\actOut$ respectively, into $1$D arrays.
Thus, the \gls{svd} dimensionality reduction and downstream steps can be applied to $\convToeplitzMatrix$.

We highlight the convolution kernels can be unrolled into a tensor of shape $\convChannelsOut\times(\convChannelsIn\times\convKernelHeight\times\convKernelWidth)$ ad proposed in \cite{praggastis2022svd}, yielding a compact matrix for the \gls{svd} compression.
However, the activations need to be unrolled into tensors of shape $(\convChannelsIn\times\convKernelHeight\times\convKernelWidth)\times(\convChannelsOut\times\convOutputHeight\times\convOutputWidth)$ yielding \corevectors with shape $\coreVecSize\times\convOutputHeight\times\convOutputWidth$, which can be detrimental to the \gls{hlf} association step.
Thus, we adopt the Toeplitz unrolling herein described due to its broader applicability within the models studied in this paper.

\subsubsection{Extension for Vision Transformers}\label{subsec: vit extension}

In order to investigate the internal representations of the \gls{vit} \cite{dosovitskiy2020image}, we restrict our analysis to the embedding associated with the  \codeFont{<cls>} token.
This choice is motivated by two considerations.
First, the  \codeFont{<cls>} token provides a global representation of the input image: through the self-attention mechanism, it aggregates contextual information from all patch embeddings at each encoder layer. 
Second, the  \codeFont{<cls>} embedding is of particular importance for downstream prediction, as it is the sole token used by the classification head to produce the final output. 
By analyzing these activations across layers, we obtain a layer-wise characterization of how the \codeFont{<cls>} token evolves throughout the network and how global image representations are progressively refined to support classification.

\section{Dataset overview}\label{app: dataset}

\rev{add intro text}
For each intensity, we subsample approximately $\left\lfloor10{,}000/13\right\rfloor$ images per corruption type, leading to a balanced test set of $10{,}000$ images in total.

which is sub-sampled to $10{,}000$ images for $\validationSet$ and another $10{,}000$ for $\testSet$ for comparison purposes

\begin{table}[h]
	\centering
	\caption{
		Summary of Datasets Used in Experiments. Each dataset is divided intro three splits, namely train ($\trainingSet$), validation ($\validationSet$), and test ($\testSet$).
		$\trainingSet$ is used for tuning the model to each dataset (Section \ref{subsec: models}), for fitting the \gls{gmm}, computing $\empiricalPosterior$, and creating the \protoclasses; $\validationSet$ is used for tuning the $\coreVecSize, \numClusters$ hyper-parameters, and $\testSet$ to evaluate the proposed framework. 
	}
	\label{tab: datasets}
	\begin{tabulary}{\linewidth}{LCCCC}
		\toprule
		\textbf{Dataset} & \textbf{Input Shape ($\img$)} & $\trainingSetSize$ & $\validationSetSize$ & $\testSetSize$ \\ 
		\midrule
		\cifar{10} & $32 \times 32 \times 3$ & $40,000$ & $10,000$ & $10,000$ \\ 
		\cifar{100} & $32 \times 32 \times 3$ & $40,000$ & $10,000$ & $10,000$ \\ 
		\cifar{100C} & $32 \times 32 \times 3$ & - & $10,000$ & $10,000$ \\
		\places & $256 \times 256 \times 3$ & - & $10,000$ & $10,000$ \\
		\SVHN & $32 \times 32 \times 3$ & - & $10,000$ & $10,000$ \\
		% \imagenet & $224 \times 224 \times 3$ & 1,281,167 & - & 50,000\\ 
		\bottomrule
	\end{tabulary}%
\end{table}

\section{Layers overview}\label{app: layers overview}

\rev{add intro text}

\begin{table}[ht]
	\centering
	\caption{Dimensions and Types of Selected Layers in \vit{B}{16} for each of the 12 encoders}
	\label{tab:vit_selected_layers}
	\begin{tabular}{l l r}
		\toprule
		\textbf{Layer} & \textbf{Type} & \textbf{$\actInSize$} \\ 
		\midrule
		\codeFont{mlp.\rev{X}.0} & \codeFont{Dense} & $768$ \\
		\codeFont{mlp.\rev{X}.3} & \codeFont{Dense} & $3072$ \\
		\texttt{heads.head} & \codeFont{Dense} & $768$ \\
		\bottomrule
	\end{tabular}%
\end{table}

\begin{table}[ht]
	\centering
	\caption{Dimensions and Types of Selected Layers in \vgg{16}}
	\label{tab:vgg16_selected_layers}
	\begin{tabular}{l l p{2.cm} r}
		\toprule
		\textbf{Layer} & \textbf{Type} & \textbf{$\convInputHeight\times\convInputWidth\times\convChannelsIn$} & \textbf{$\actInSize$} \\ 
		\midrule
		\codeFont{f.7} & \codeFont{Conv2D} & $112 \times 112 \times 128$ & $1,605,632$ \\ 
		\codeFont{f.10} & \codeFont{Conv2D} & $56 \times 56 \times 128$ & $401,408$ \\ 
		\codeFont{f.12} & \codeFont{Conv2D} & $56 \times 56 \times 256$ & $802,816$ \\ 
		
		\codeFont{f.14} & \codeFont{Conv2D} & $56 \times 56 \times 256$ & $802,816$ \\
		\codeFont{f.17} & \codeFont{Conv2D} & $28 \times 28 \times 256$ & $200,704$ \\
		\codeFont{f.19} & \codeFont{Conv2D} & $28 \times 28 \times 512$ & $401,408$ \\
		\codeFont{f.21} & \codeFont{Conv2D} & $28 \times 28 \times 512$ & $401,408$ \\
		
		\codeFont{f.24} & \codeFont{Conv2D} & $14 \times 14 \times 512$ & $100,352$ \\ 
		\codeFont{f.26} & \codeFont{Conv2D} & $14 \times 14 \times 512$ & $100,352$ \\ 
		\codeFont{f.28} & \codeFont{Conv2D} & $14 \times 14 \times 512$ & $100,352$ \\ 
		\codeFont{c.0} & \codeFont{Dense} & - & $25,088$ \\ 
		\codeFont{c.3} & \codeFont{Dense} & - & $4,096$ \\ 
		\codeFont{c.6} & \codeFont{Dense} & - & $4,096$ \\
		\bottomrule
	\end{tabular}%
\end{table}

\section{Adversaria Attacks Setup}\label{app: atks hyper-parameters}

The distance metrics \rev{parameters?} used for the generation of adversarial examples are $\ell_2$ for \gls{df} and \gls{cw} and $\ell_{\rm inf}$ for \gls{pgd} and \gls{bim}.

\rev{@Lorenzo, can we have the parameters and their success rate?}

\section{Hyper-parameters Tuning}\label{app: Hyperparameters tuning}

The values for $\coreVecSize$ and $\numClusters$ found by \ray are reported on Table \ref{tab: tuning configs}.

\begin{table}
	\caption{Best $\coreVecSize, \numClusters$ configuration found through hyper-parameter tuning.}
	\label{tab: tuning configs}
	\begin{subtable}[t]{0.45\linewidth}
		\centering
		\caption{\vgg{16}}
		\begin{tabular}[t]{lcc}
			\toprule
			& $\coreVecSize$ & $\numClusters$ \\\midrule
			\codeFont{f.7} & 500 & 1360 \\ 
			\codeFont{f.10} & 479 & 2239 \\ 
			\codeFont{f.12} & 442 & 2159  \\ 
			\codeFont{f.14} & 496 & 524  \\
			\codeFont{f.17} & 356 & 773  \\
			\codeFont{f.19} & 499 & 1326  \\
			\codeFont{f.21} & 489 & 851  \\
			\codeFont{f.24} & 323 & 1035  \\ 
			\codeFont{f.26} & 351 & 838  \\ 
			\codeFont{f.28} & 377 & 1481  \\ 
			\codeFont{c.0} & 50 & 1717  \\ 
			\codeFont{c.3} & 53 & 1627  \\ 
			\codeFont{c.6} & 51 & 1706  \\
			\bottomrule
		\end{tabular}
	\end{subtable}
	\begin{subtable}[t]{0.45\linewidth}
		\centering
		\caption{\vit{B}{16}}
		\begin{tabular}[t]{lcc}
			\toprule 
			& $\coreVecSize$ & $\numClusters$ \\\midrule
			\codeFont{mpl.0.0} & 448 & 1694 \\
			\codeFont{mpl.1.0} & 52 & 2436 \\
			\codeFont{mpl.2.0} & 390 & 1527 \\ 
			\codeFont{mpl.3.0} & 100 & 1881 \\ 
			\codeFont{mpl.4.0} & 156 & 2295 \\ 
			\codeFont{mpl.5.0} & 174 & 1761 \\ 
			\codeFont{mpl.6.0} & 254 & 1945 \\ 
			\codeFont{mpl.7.0} & 253 & 1234 \\ 
			\codeFont{mpl.8.0} & 376 & 1025 \\ 
			\codeFont{mpl.9.0} & 500 & 918 \\ 
			\codeFont{mpl.10.0} & 258 & 1060 \\ 
			\codeFont{mpl.11.0} & 378 & 3714 \\ 
			
			\codeFont{mpl.0.3} & 54 & 1417 \\ 
			\codeFont{mpl.1.3} & 83 & 3252 \\
			\codeFont{mpl.2.3} & 469 & 1423 \\
			\codeFont{mpl.3.3} & 333 & 2921 \\
			\codeFont{mpl.4.3} & 405 & 1606 \\
			\codeFont{mpl.5.3} & 398 & 1321 \\
			\codeFont{mpl.6.3} & 410 & 2381 \\
			\codeFont{mpl.7.3} & 479 & 1766 \\
			\codeFont{mpl.8.3} & 346 & 1486 \\
			\codeFont{mpl.9.3} & 441 & 1263 \\
			\codeFont{mpl.10.3} & 403 & 2473 \\
			\codeFont{mpl.11.3} & 153 & 2373 \\
			\codeFont{heads.head} & 52 & 4519 \\ 
			\bottomrule
		\end{tabular}
	\end{subtable}
\end{table}

The \vgg{16}\footnote{The layer naming convention adopted in this work follows the structure defined in \torchVision, where convolutional layers are grouped under \codeFont{features} and fully connected layers are part of the \codeFont{classifier} block.} results show an interesting trend on the $\coreVecSize$, which starts high ($\approx500$) for the early convolutional layers until \codeFont{f.21}, become smaller for the later $3$ convolutional layers ($\approx350$), and are significantly small for the linear layers ($\approx50$).
The direct correlation with the layer's dimension (Table \ref{tab:vgg16_selected_layers}) indicates that the early layers encode a higher number of \gls{llf}, making it necessary to increase $\coreVecSize$ in order to cope with the amount of information.
On the other hand, \vit{B}{16} we notice a tendency of \codeFont{mlp.\rev{X}.0} layers to require smaller $\coreVecSize$s than their respective \codeFont{mlp.\rev{X}.3} counter-part \rev{are these the key, query, and something else?}.

Regarding the $\numClusters$, we see a greater variance, which is expected since increasing the number of clusters implies dividing clusters into nearby smaller ones.
Nevertheless, it is interesting to note that the number seldom surpasses $\numClusters=2500$, which we speculate to be limit by the data availability and diversity given that increasing $\numClusters$ lead to a more sparse $\empiricalPosterior$ representation.

As a note for future work, the $\numClusters$ values found can indicate an estimate on the number of \gls{llf} encoded in the model.

\section{Reference Method's Hyper-parameters}\label{subapp: reference methods hyperp}

\rev{describe here the ranges, procedure and found values for \gls{doc} and \gls{relu}. Does \gls{dmd} has hyperparams? also for \gls{fs}}

\section{Example \codeFont{Classification-maps}}\label{app: other conceptos}

\rev{Add other interesting conceptograms, discuss how the highlighted classes have similar meaning, discuss their protoclasses and conceptograms, predictions and scores}

\section{Results classification maps}\label{app: tuning DMD base}

\textbf{ViT}

\begin{table}[htbp]
\centering
\caption{DMD-B Out-of-Distribution AUCs for ViT on CIFAR-100}
\label{tab:dmd_ood_aucs}
\pgfplotstabletypeset[
    col sep=comma,
    columns/magnitude/.style={column name=\textbf{Magnitude}, fixed, precision=3},
    columns/Places365-val/.style={column name=\textbf{Places365-val}, fixed, precision=2},
    columns/SVHN-val/.style={column name=\textbf{SVHN-val}, fixed, precision=2},
    columns/meanAUC/.style={column name=\textbf{Mean AUC}, fixed, precision=2},
    every head row/.style={before row=\toprule, after row=\midrule},
    every last row/.style={after row=\bottomrule},
]{figures/cifar100_ViT/DMDbase/tuningOOD.csv}
\end{table}

\begin{table}[htbp]
\centering
\caption{DMD-B Atks AUCs for ViT on CIFAR-100}
\label{tab:dmd_ood_aucs}
\pgfplotstabletypeset[
    col sep=comma,
    columns/magnitude/.style={column name=\textbf{Magnitude}, fixed, precision=3},
    columns/BIM/.style={column name=\textbf{BIM}, fixed, precision=2},
    columns/CW/.style={column name=\textbf{CW}, fixed, precision=2},
    columns/DF/.style={column name=\textbf{DF}, fixed, precision=2},
    columns/PGD/.style={column name=\textbf{PGD}, fixed, precision=2},
    columns/meanAUC/.style={column name=\textbf{Mean AUC}, fixed, precision=2},
    every head row/.style={before row=\toprule, after row=\midrule},
    every last row/.style={after row=\bottomrule},
]{figures/cifar100_ViT/DMDbase/tuningATK.csv}
\end{table}

\begin{table}[htbp]
\centering
\caption{DMD-B corr AUCs for ViT on CIFAR-100}
\label{tab:dmd_ood_aucs}
\pgfplotstabletypeset[
    col sep=comma,
    columns/magnitude/.style={column name=\textbf{Magnitude}, fixed, precision=3},
    columns/c0/.style={column name=\textbf{c0}, fixed, precision=2},
    columns/c1/.style={column name=\textbf{c1}, fixed, precision=2},
    columns/c2/.style={column name=\textbf{c2}, fixed, precision=2},
    columns/c3/.style={column name=\textbf{c3}, fixed, precision=2},
    columns/meanAUC/.style={column name=\textbf{Mean AUC}, fixed, precision=2},
    every head row/.style={before row=\toprule, after row=\midrule},
    every last row/.style={after row=\bottomrule},
]{figures/cifar100_ViT/DMDbase/tuningCorr.csv}
\end{table}

\begin{table}[htbp]
\centering
\caption{DMD-B conf AUCs for ViT on CIFAR-100}
\label{tab:dmd_ood_aucs}
\pgfplotstabletypeset[
    col sep=comma,
    columns/magnitude/.style={column name=\textbf{Magnitude}, fixed, precision=3},
    columns/c0/.style={column name=\textbf{c0}, fixed, precision=2},
    columns/c1/.style={column name=\textbf{c1}, fixed, precision=2},
    columns/meanAUC/.style={column name=\textbf{Mean AUC}, fixed, precision=2},
    every head row/.style={before row=\toprule, after row=\midrule},
    every last row/.style={after row=\bottomrule},
]{figures/cifar100_ViT/DMDbase/tuningConf.csv}
\end{table}

\textbf{vgg16}

\begin{table}[htbp]
\centering
\caption{DMD-B Out-of-Distribution AUCs for vgg16 on CIFAR-100}
\label{tab:dmd_ood_aucs}
\pgfplotstabletypeset[
    col sep=comma,
    columns/magnitude/.style={column name=\textbf{Magnitude}, fixed, precision=3},
    columns/Places365-val/.style={column name=\textbf{Places365-val}, fixed, precision=2},
    columns/SVHN-val/.style={column name=\textbf{SVHN-val}, fixed, precision=2},
    columns/meanAUC/.style={column name=\textbf{Mean AUC}, fixed, precision=2},
    every head row/.style={before row=\toprule, after row=\midrule},
    every last row/.style={after row=\bottomrule},
]{figures/cifar100_vgg16/DMDbase/tuningOOD.csv}
\end{table}

\begin{table}[htbp]
\centering
\caption{DMD-B Atks AUCs for vgg16 on CIFAR-100}
\label{tab:dmd_ood_aucs}
\pgfplotstabletypeset[
    col sep=comma,
    columns/magnitude/.style={column name=\textbf{Magnitude}, fixed, precision=3},
    columns/BIM/.style={column name=\textbf{BIM}, fixed, precision=2},
    columns/CW/.style={column name=\textbf{CW}, fixed, precision=2},
    columns/DF/.style={column name=\textbf{DF}, fixed, precision=2},
    columns/PGD/.style={column name=\textbf{PGD}, fixed, precision=2},
    columns/meanAUC/.style={column name=\textbf{Mean AUC}, fixed, precision=2},
    every head row/.style={before row=\toprule, after row=\midrule},
    every last row/.style={after row=\bottomrule},
]{figures/cifar100_vgg16/DMDbase/tuningATK.csv}
\end{table}

\begin{table}[htbp]
\centering
\caption{DMD-B corr AUCs for vgg16 on CIFAR-100}
\label{tab:dmd_ood_aucs}
\pgfplotstabletypeset[
    col sep=comma,
    columns/magnitude/.style={column name=\textbf{Magnitude}, fixed, precision=3},
    columns/c0/.style={column name=\textbf{c0}, fixed, precision=2},
    columns/c1/.style={column name=\textbf{c1}, fixed, precision=2},
    columns/c2/.style={column name=\textbf{c2}, fixed, precision=2},
    columns/c3/.style={column name=\textbf{c3}, fixed, precision=2},
    columns/meanAUC/.style={column name=\textbf{Mean AUC}, fixed, precision=2},
    every head row/.style={before row=\toprule, after row=\midrule},
    every last row/.style={after row=\bottomrule},
]{figures/cifar100_vgg16/DMDbase/tuningCorr.csv}
\end{table}

\begin{table}[htbp]
\centering
\caption{DMD-B conf AUCs for vgg16 on CIFAR-100}
\label{tab:dmd_ood_aucs}
\pgfplotstabletypeset[
    col sep=comma,
    columns/magnitude/.style={column name=\textbf{Magnitude}, fixed, precision=3},
    columns/c0/.style={column name=\textbf{c0}, fixed, precision=2},
    columns/c1/.style={column name=\textbf{c1}, fixed, precision=2},
    columns/meanAUC/.style={column name=\textbf{Mean AUC}, fixed, precision=2},
    every head row/.style={before row=\toprule, after row=\midrule},
    every last row/.style={after row=\bottomrule},
]{figures/cifar100_vgg16/DMDbase/tuningConf.csv}
\end{table}
